# Supplementary material for: Confidence Regions Near Singular Information and Boundary Points With Applications to Mixed Models
Source: arXiv:2103.10236 ancillary file (2022-02-01)
Supplement: Supplementary file 1 [file conf_crit_suppl.pdf]

# Supplement to “Confidence Regions Near Singular Information and Boundary Points With Applications to Mixed Models”

Karl Oskar Ekvall   Matteo Bottai

Division of Biostatistics, Institute of Environmental Medicine, Karolinska Institutet

`karl.oskar.ekvall@ki.se`   `matteo.bottai@ki.se`

February 1, 2022

## A Logistic mixed model with asymmetric random effect

### A.1 Definitions and important quantities

Let  $Y_{ij} \in \{0, 1\}$ ,  $i = 1, \dots, n$ ,  $j = 1, \dots, r$  be conditionally independent given a vector of random effects

$$W = [W_1, \dots, W_n]^T \in \mathbb{R}^n.$$

We consider a logistic generalized linear mixed model which assumes the conditional densities are

$$f_{\theta}(y_{ij} \mid w_i) = \exp\{y_{ij}(\psi + \lambda w_i) - c(\psi + \lambda w_i)\},$$

where  $c(t) = \log\{1 + \exp(t)\}$  is the cumulant function for the Bernoulli distribution. To illustrate how our method applies in setting where the critical point is not a boundary point, suppose the elements of  $W$  are independent with exponential distributions with unit rate, centered to have mean zero; that is,

$$W_i + 1 \sim \text{Exp}(1), \quad i = 1, \dots, n.$$

We denote the distribution of  $W_i$  by  $\nu$  and note it has Lebesgue density  $f(w_i) = \exp\{-(w_i+1)\}$  on  $(-1, \infty)$ . The parameter is  $\theta = (\lambda, \psi)$  and the parameter set is  $\Theta = \mathbb{R}^2$ . A straightforward calculation shows  $\mathbb{E}_{\theta}(Y_{ij} \mid W) = c'(\psi + \lambda W_i) = 1/\{1 + \exp(-\psi - \lambda W_i)\}$ , where the prime denotes derivative.

This model could be used, for example, for inference on the prevalence of some disease using test results for  $nr$  patients, where patients with the same index  $i$  are from the same test location. Then the random effect is used to model an asymmetric location effect which, if  $\lambda \neq 0$ , implies observations from the same location are dependent. Location effects often thought to be asymmetric include, for example, ones due to pollution. Continuing with that example, the probability that a randomly selected patient has the disease is

$$\mathbb{E}_\theta(Y_{ij}) = \mathbb{E}_\theta\{\mathbb{E}_\theta(Y_{ij} \mid W)\} = \mathbb{E}_\theta\{c'(\psi + \lambda W_i)\} = \int \frac{1}{1 + \exp(-\psi - \lambda w_i)} \nu(dw_i).$$

Inference on this probability requires inference on both  $\psi$  and  $\lambda$ , which we will consider using a (joint) confidence region for  $(\lambda, \psi)$ .

Before presenting simulations and a synthetic data analysis, we state some important quantities and briefly discuss how they can be computed in practice. Let  $y^n = [y_{11}, \dots, y_{nr}]^\top$  be a vector of all observations and  $y_i = [y_{i1}, \dots, y_{ir}]^\top$ . The log-likelihood is

$$\ell_n(\theta; y^n) = \sum_{i=1}^n \log \int f_\theta(y_i \mid w_i) \nu(dw_i),$$

where, due to conditional independence,

$$f_\theta(y_i \mid w_i) = \prod_{j=1}^r f_\theta(y_{ij} \mid w_i).$$

Routine derivative calculations give the score function

$$s_n(\theta; y^n) = \sum_{i=1}^n \frac{1}{f_\theta(y_i)} \int f_\theta(y_i \mid w_i) \{y_{i\bullet} - r c'(\psi + \lambda w_i)\} \begin{bmatrix} w_i \\ 1 \end{bmatrix} \nu(dw_i)$$

where  $y_{i\bullet} = \sum_{j=1}^r y_{ij}$  and

$$f_\theta(y_i) = \int f(y_i \mid w_i) \nu(dw_i) = \mathbf{P}_\theta(Y_i = y_i).$$

To evaluate these integrals in practice we use numerical quadrature rules for integrals with respect to the exponential distribution, with 10 nodes using the **statmod** R package (Smyth, 1998).

Because the vectors  $Y_i = [Y_{i1}, \dots, Y_{ir}]^\top$  are independent and identically distributed, the

Fisher information is

$$\mathcal{I}_n(\theta) = n\mathbb{E}_\theta [s^1(\theta; Y_1)s^1(\theta; Y_1)^\top] = n \sum_{y \in \{0,1\}^r} \mathbb{P}_\theta(Y_1 = y) s^1(\theta; y) s^1(\theta; y)^\top,$$

where the sum is taken over all elements in the support of  $Y_1$ .

Our theory implies every point where  $\lambda = 0$  is a critical point. Indeed, as discussed in Section 3 of the main text, at every such point  $e_1 = [1, 0]^\top$  is an eigenvector of the Fisher information with eigenvalue zero. However, unlike the examples in the main text, there are no boundary points in this setting since  $\Theta = \mathbb{R}^2$ .

To evaluate the proposed test-statistic at the critical points, define

$$\bar{s}_n(\theta; y^n) = \begin{cases} s_n(\theta; y^n) & \lambda \neq 0 \\ [\nabla_\lambda^2 \ell_n(\theta; y^n), \nabla_\psi \ell_n(\theta; y^n)]^\top & \lambda = 0 \end{cases}.$$

As remarked in Section 3 of the main text, we have

$$T_n(\theta; y^n) = \tilde{s}_n(\theta; y^n)^\top \tilde{\mathcal{I}}_n(\theta)^{-1} \tilde{s}_n(\theta; y^n) = \bar{s}_n(\theta; y^n)^\top \text{cov}_\theta\{\bar{s}_n(\theta; Y^n)\}^{-1} \bar{s}_n(\theta; y^n).$$

In the notation of the general theory in Section 2 of the main text, our choice of  $\bar{s}_n$  corresponds to taking  $k_1(\theta) = k_2(\theta) = 1$  at every  $\theta$  such that  $\lambda \neq 0$ , and  $k_1(\theta) = 2$  and  $k_2(\theta) = 1$  at  $\theta$  where  $\lambda = 0$ , reflecting the fact that  $e_1$  is a critical vector.

To get an expression for  $\bar{s}_n$  that can be evaluated in practice, differentiate the first element of  $s_n(\theta; y^n)$  with respect to  $\lambda$  to get

$$\begin{aligned} \nabla_\lambda^2 \ell_n(\theta; y^n) &= \sum_{i=1}^n -\frac{1}{f_\theta(y_i)^2} \left[ \int f_\theta(y_i | w_i) \{y_{i\bullet} - rc'(\psi + \lambda w_i)\} w_i \nu(dw_i), \right]^2 \\ &+ \sum_{i=1}^n \frac{1}{f_\theta(y_i)} \int f_\theta(y_i | w_i) \left[ \{y_{i\bullet} - rc'(\psi + \lambda w_i)\}^2 - rc''(\psi + \lambda w_i) \right] w_i^2 \nu(dw_i). \end{aligned}$$

The first sum on the right-hand side is  $\sum_{i=1}^n s_\lambda^i(\theta; y_i)^2$ , which is zero at points where  $\lambda = 0$ . Thus, when  $\lambda = 0$ ,

$$\nabla_\lambda^2 \ell_n(\theta; y^n) = \sum_{i=1}^n \frac{1}{f_\theta(y_i)} \int f_\theta(y_i | w_i) \left[ \{y_{i\bullet} - rc'(\psi + \lambda w_i)\}^2 - rc''(\psi + \lambda w_i) \right] w_i^2 \nu(dw_i),$$

which is straightforward to evaluate using numerical quadrature. Upon inspecting the

integrands it is clear the computational cost of evaluating  $\nabla_\lambda^2 \ell(\theta; y^n)$  when  $\lambda = 0$  is roughly equivalent to that of evaluating  $\nabla_\lambda \ell_n(\theta; y^n)$  when  $\lambda \neq 0$ . Similarly, the cost of evaluating  $\text{cov}_\theta\{\bar{s}(\theta; Y^n)\}$  when  $\lambda = 0$  is similar to the cost of evaluating  $\mathcal{I}_n(\theta)$  when  $\lambda \neq 0$  since

$$\text{cov}_\theta\{\bar{s}(\theta; Y^n)\} = n \text{cov}_\theta\{\bar{s}^1(\theta; Y_1)\} = n \sum_{y \in \{0,1\}^r} \mathbb{P}_\theta(Y_1 = y) \bar{s}^1(\theta; y) \bar{s}^1(\theta; y)^\top.$$

## A.2 Coverage simulations

We examine coverage probabilities of parameters in a neighborhood of a critical point. Specifically, we generate data with  $\psi = 0.5$  and

$$\lambda \in \{0, \pm 10^{-6}, \pm 0.01, \pm 0.05, \pm 0.1, \pm 0.25, \pm 0.4, \pm 0.55, \pm 0.7, \pm 0.85, \pm 1\}.$$

To provide context we, in addition to our method, consider coverage of confidence regions obtained by inverting likelihood-ratio and Wald test-statistics. Specifically, let

$$T_n^L(\theta; y^n) = 2\{\ell_n(\hat{\theta}; y^n) - \ell_n(\theta; y^n)\},$$

where  $\hat{\theta} \in \arg \max_{\theta \in \Theta} \ell_n(\theta; y^n)$ . Let also

$$T_n^W(\theta; y^n) = (\hat{\theta} - \theta)^\top \mathcal{I}_n(\hat{\theta})(\hat{\theta} - \theta).$$

The confidence regions are  $\mathcal{R}_n(\alpha) = \{\theta \in \mathbb{R}^2 : T_n(\theta; y^n) \leq q_{2,1-\alpha}\}$ ,  $\mathcal{R}_n^L(\alpha) = \{\theta \in \mathbb{R}^2 : T_n^L(\theta; y^n) \leq q_{2,1-\alpha}\}$ , and  $\mathcal{R}_n^W(\alpha) = \{\theta \in \mathbb{R}^2 : T_n^W(\theta; y^n) \leq q_{2,1-\alpha}\}$ ; where  $q_{2,1-\alpha}$  is the  $(1 - \alpha)$ th quantile of the chi-square distribution with 2 degrees of freedom. For our test-statistic the reference distribution is motivated by the asymptotic theory in the main text. For  $T_n^L$  and  $T_n^W$  it is motivated for interior points of the parameter set by classical asymptotic theory (e.g. Ferguson, 1996). However, that theory typically does not apply when the Fisher information is singular, so we expect potentially poor coverage near critical points.

We obtained  $\hat{\theta}$  by applying the off-the-shelf optimizer `optim` in R to our implementation of the log-likelihood. Some further remarks on computing and the associated times are in Section B.

Figure A presents results for  $n \in \{20, 80\}$  and  $r = 5$  based on 10,000 Monte Carlo replications. Notably, coverage for the proposed method is near-nominal for all settings while coverage for the other methods depends on how close to zero the true  $\lambda$  is and what the sample size  $n$  is. In summary, the simulations indicate the asymptotic theory under a

sequence of parameters gives useful guidance on coverage properties in finite samples.

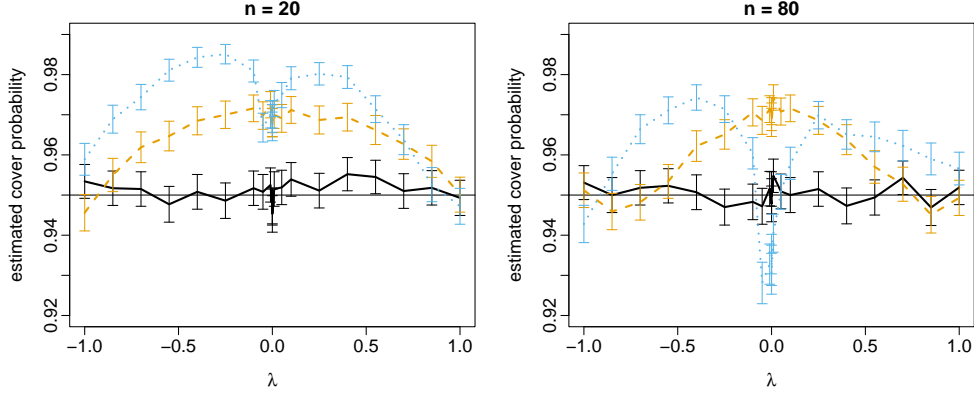

Figure A: Monte Carlo estimates of coverage probabilities of confidence regions from inverting the proposed (solid), likelihood ratio (dashed), and Wald (dotted) test-statistics. The straight horizontal line indicates the nominal 0.95 coverage probability and vertical bars denote  $\pm 2$  times Monte Carlo standard errors.

### A.3 Synthetic data analysis

To illustrate how the method can be applied in practice, we considered one synthetic dataset like those in the simulations, with  $n = 80$ ,  $r = 5$ ,  $\psi = 0.5$ , and  $\lambda = -0.5$ . We created a confidence region for  $(\lambda, \psi)$  by inverting the proposed test statistic (Figure B) numerically. More specifically, we evaluated the test-statistic at a grid of 50 values each of  $\lambda$  and  $\psi$ , meaning 2500 evaluations in total and included in the confidence region those  $\theta$  for which  $T_n(\theta; y^n) \leq q_{2,1-\alpha}$ . To get an idea of where to center that grid we maximized an approximation to the likelihood based on numerical quadrature with just one node. This gave fast and reasonable guidance on which values to consider for the inversion. We got the maximizing point  $(\tilde{\lambda}, \tilde{\psi}) = (-0.044, 0.55)$  and, based on this, centered the grid at  $(0, 0.5)$ . Similarly, to get a rough idea for how large to make the grid, one may first compute an inexact Wald-type confidence region based on a fast approximation of the likelihood or evaluate componentwise test-statistics at a few values to get a rough idea of ranges of parameter values to consider. Typically, a few evaluations per parameter is sufficient and, hence, the computational effort of this step is negligible in comparison to evaluating the test-statistic on the resulting grid. In many settings, subject-specific knowledge may also inform which parameter values to consider.

Figure B shows the confidence region includes both positive and negative values of  $\lambda$ .

However, the region is not symmetric around the line  $\lambda = 0$ , which it would be if the random effect were symmetrically distributed around zero.

To make inferences about  $\mathbb{E}_\theta(Y_{ij}) = \mathbb{P}_\theta(Y_{ij} = 1)$ , which is the same for all  $i$  and  $j$ , we numerically calculated the image of the 95% region in Figure B under the mapping  $\theta \mapsto \mathbb{E}_\theta(Y_{ij})$ . Specifically, we calculated  $\mathbb{E}_\theta(Y_{ij})$  for all  $\theta$  in our grid which satisfied  $T_n(\theta; y^n) \leq q_{2,0.95}$  and then computed the range of those numbers. This gave the interval  $(0.58, 0.69)$ , which includes the true value  $0.62 = \int c'(0.5 - 0.5w_i)\nu(dw_i)$ .

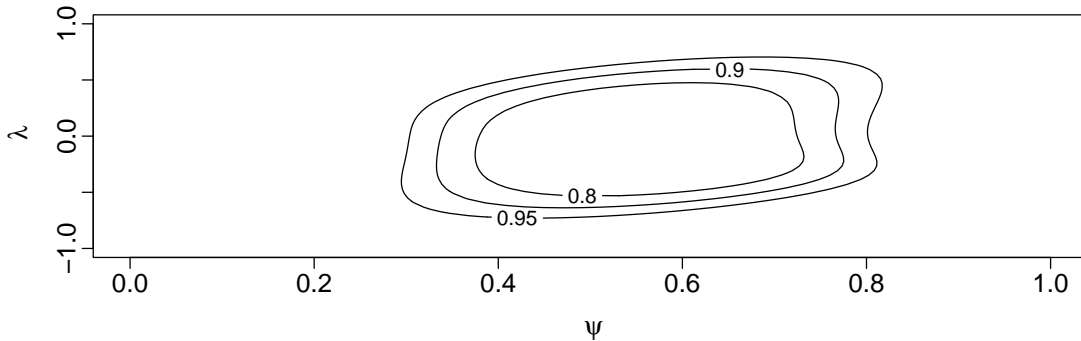

Figure B: Joint 80–95 % confidence regions for  $(\lambda, \psi)$ , based on the proposed test-statistic and the chi-square distribution with 2 degrees of freedom.

## B Computing times

Tables A and C show average computing times for the proposed test-statistic and the likelihood ratio test statistic, for the linear mixed model simulations in the main text and the logistic mixed model simulations presented earlier, respectively. We do not report times for the Wald statistic because they were essentially the same as for the likelihood-ratio statistic; for either, most of the time is spent calculating the maximum likelihood estimates. For brevity we report times for a subset of the considered parameter values; times were similar for the parameter values not reported. All times are on a MacBook Pro with 2.6 GHz 6-core Intel i7 CPU.

In all of our simulation settings, the proposed test-statistic was on average substantially faster to compute than the other two. However, we caution the reader that it is not possible to say which test-statistic is faster to compute in general. In some settings computing the Fisher information is computationally cheaper than obtaining maximum likelihood estimates, but it is easy to come up with a setting where that is not the case. Thus, in some settings there will be a trade-off between computing costs and the properties of the test statistics.

We expect the particular implementation one is using to have a substantial effect on computing times. For example, for the model in Section A we used a naive implementation of numerical integration in R to evaluate our test-statistic and we used the off-the-shelf optimizer `optim` to get the maximum likelihood estimates. We considered both derivative free and quasi-Newton optimization (L-BFGS-B) and times were similar. Optimized implementations in a compiled language (e.g. Fortran, C, or C++) would likely speed up all methods by orders of magnitude.

Computing when there are many, potentially crossed, random effects in a non-linear model poses additional challenges. Indeed, even evaluating the likelihood in such settings is complicated. Some Monte Carlo-based methods have been proposed (Knudson et al., 2021) and these could potentially be adapted to our method, possibly in conjunction with existing methods for evaluating the Fisher information matrix using Monte Carlo (Riviere et al., 2016). In practice it is more common, however, not to evaluate the likelihood at all and instead use a fast but potentially inaccurate approximation. For example, when there are more than one random effect the `lme4` package bases inference on a Laplace approximation of the likelihood, which is equivalent to adaptive Gaussian quadrature with one node. Similar approaches are taken in other common software and could be implemented for the integrals required by our method.

Inverting the proposed test-statistic or the likelihood ratio test-statistic in practice can require evaluating them many times. For example, we evaluated the test statistic 2500 times in our data example in Section A, and this took about 39 seconds using a single CPU core. In higher dimensions computing times will increase substantially. On the other hand, the time required for numerical inversion can be decreased if several cores are available since the test-statistics can be evaluated at different points in parallel.

| (a) $n = 20$ |           |      |      | (b) $n = 80$ |           |        |        |
|--------------|-----------|------|------|--------------|-----------|--------|--------|
|              | $\lambda$ |      |      |              | $\lambda$ |        |        |
|              | 0         | 0.01 | 0.5  |              | 0         | 0.01   | 0.5    |
| our          | 1.65      | 1.50 | 1.50 | our          | 98.01     | 82.94  | 78.63  |
| lrt          | 4.28      | 3.82 | 4.94 | lrt          | 299.72    | 264.50 | 232.05 |

Table A: Average computing times (100th of s.) for linear mixed model over 10,000 Monte Carlo replications.

|     | (a) $n = 20$ |      |      |     | (b) $n = 80$ |       |       |
|-----|--------------|------|------|-----|--------------|-------|-------|
|     | $\lambda$    |      |      |     | $\lambda$    |       |       |
|     | 0            | 0.01 | 0.55 |     | 0            | 0.01  | 0.55  |
| our | 1.08         | 0.91 | 0.93 | our | 2.90         | 2.47  | 2.50  |
| lrt | 9.52         | 8.63 | 9.51 | lrt | 33.25        | 29.17 | 31.18 |

Table C: Average computing times (100th of s.) for logistic mixed model over 10,000 Monte Carlo replications.

## C Details for Example 1

Recall, the  $Y_i = [Y_1, \dots, Y_r]^\top$ ,  $i = 1, \dots, n$ , are independent and multivariate normally distributed with mean 0 and common covariance matrix  $\Sigma(\theta) = \theta^2 \mathbf{1}_r \mathbf{1}_r^\top + I_r$ . Thus, the log-likelihood is for one observation is

$$\log f_\theta(y_i) = -\frac{1}{2} \log |\Sigma(\theta)| - \frac{1}{2} y_i^\top \Sigma(\theta)^{-1} y_i.$$

Since  $\mathbf{1}_r \mathbf{1}_r^\top$  has eigenvalues  $r$  and 0,  $\Sigma(\theta)$  has eigenvalues  $1 + r\theta^2$  and 1, the latter with multiplicity  $r - 1$ . Thus,  $|\Sigma(\theta)| = (1 + r\theta^2)1^{r-1} = 1 + r\theta^2$ . Applying the Sherman–Morrison formula to  $\Sigma(\theta)^{-1}$  gives  $(I_r + \theta^2 \mathbf{1}_r \mathbf{1}_r^\top)^{-1} = I_r - \theta^2 \mathbf{1}_r \mathbf{1}_r^\top (1 + r\theta^2)^{-1}$ , and hence  $2 \log f_\theta(y_i) = -\log(1 + r\theta^2) - y_i^\top y_i + (y_i^\top \mathbf{1}_r)^2 \theta^2 (1 + r\theta^2)^{-1}$ . Differentiating  $\log f_\theta(y_i)$  with respect to  $\theta$  gives  $s^i(\theta; y_i) = -r\theta(1 + r\theta^2)^{-1} + \theta(y_i^\top \mathbf{1}_r)^2(1 + r\theta^2)^{-2}$ . Differentiating again we get  $h^i(\theta; y_i) = -(r - r^2\theta^2)\{(1 + r\theta^2)^2\}^{-1} + (y_i^\top \mathbf{1}_r)^2(1 - 3r\theta^2)(1 + r\theta^2)^{-3}$ . Thus, using that  $\mathbb{E}_\theta\{(Y_i^\top \mathbf{1}_r)^2\} = \text{var}_\theta(Y_i^\top \mathbf{1}_r) = \mathbf{1}_r^\top \Sigma(\theta) \mathbf{1}_r = \mathbf{1}_r^\top \mathbf{1}_r (1 + r\theta^2) = r(1 + r\theta^2)$  we find  $\mathcal{I}^i(\theta) = -\mathbb{E}_\theta[h^i(\theta; Y_i)] = (r - r^2\theta^2)(1 + r\theta^2)^{-2} - r(1 + r\theta^2)(1 - 3r\theta^2)(1 + r\theta^2)^{-3} = 2r^2\theta^2(1 + r\theta^2)^{-2}$ . Consequently, for  $\theta > 0$ ,

$$T_n(\theta; y^n)^{1/2} = n^{-1/2} \sum_{i=1}^n \frac{s^i(\theta; y_i)}{\sqrt{\mathcal{I}^1(\theta)}} = (2n)^{-1/2} \sum_{i=1}^n \left\{ -1 + \frac{(y_i^\top \mathbf{1}_r)^2}{r(1 + r\theta^2)} \right\}.$$

Define the score test-statistic standardized by observed information

$$T_n^O(\theta; y^n) = s_n(\theta; y^n)^\top \left\{ -\nabla^2 \ell_n(\theta; y^n) \right\}^{-1} s_n(\theta; y^n).$$

**Theorem C.1.** *In Example 1, with known  $\psi = 0$  and  $r = 1$  it holds as  $n \rightarrow \infty$ , with*

$Z \sim \mathcal{N}(0, 1)$ ,

$$T_n^O(\theta_n; Y_n^n) \rightsquigarrow \begin{cases} Z^2 & \text{if } n^{1/4}|\theta_n| \rightarrow \infty \\ \frac{2a^2 Z^2}{2a^2 - \sqrt{2}Z} & \text{if } \theta_n = an^{-1/4}, \quad a \in \mathbb{R}, \\ 0 & \text{if } \theta_n = o(n^{-1/4}) \end{cases}$$

where  $Y_n^n = (Y_{n1}, \dots, Y_{nn})$  has the distribution indexed by  $\theta_n$ .

*Proof.* Recall  $s^i(\theta; y_i) = \theta\{-1 + y_i^2/(1 + \theta^2)\}/(1 + \theta^2)$ . Some algebra gives that  $\nabla^2 \ell^i(\theta; y_i) = (\theta^4 - 3\theta^2 y_i^2 + y_i^2 - 1)/(1 + \theta^2)^3$  and hence

$$T_n^O(\theta; y^n) = \theta^2(1 + \theta^2) \frac{[\sum_{i=1}^n \{y_i/(1 + \theta^2) - 1\}]^2}{\sum_{j=1}^n \{1 - y_j^2 + 3\theta^2 y_j^2 - \theta^4\}}$$

Let  $x_n = \sum_{i=1}^n \{y_i^2/(1 + \theta^2) - 1\}$ , or  $\sum_{i=1}^n y_i^2 = (1 + \theta^2)(x_n + n)$ , to get

$$\begin{aligned} T_n^O(\theta; y^n) &= \theta^2(1 + \theta^2) \frac{x_n^2}{n(1 + \theta^2)(1 - \theta^2) - (1 - 3\theta^2)(x_n + n)(1 + \theta^2)} \\ &= \frac{x_n^2/n}{2 - (1 - 3\theta^2)(\theta^2 n)^{-1}x_n} \end{aligned}$$

Observe that  $X_n \sim (\chi_n^2 - n)$  regardless of  $\theta$ , where  $X_n$  is defined as  $x_n$  but with  $Y_i$  in place of  $y_i$ . Thus,  $n^{-1/2}X_n \rightsquigarrow \sqrt{2}Z$  by the central limit theorem. Thus, if  $\theta_n^2 n = a^2 \sqrt{n}$ , or  $\theta_n = an^{-1/4}$ , then  $T_n^O(\theta_n) \rightsquigarrow 2a^2 Z^2/(2a^2 - \sqrt{2}Z)$  by Slutsky and mapping theorems. The other cases now follow by routine arguments.  $\square$

## D Additional results

**Lemma D.1.** *If Assumptions 1–2 and 4–5 hold; then for any  $n = 1, 2, \dots$  and  $\{\theta_m\} \in \Theta$  tending to some  $\theta \in \Theta$ , with  $Y_m^n$  and  $Y^n$  having the distributions indexed by  $\theta_m$  and  $\theta$ , respectively, as  $m \rightarrow \infty$  with  $n$  fixed:*

$$T_n(\theta_m; Y_m^n) \rightsquigarrow T_n(\theta; Y^n).$$

*Proof.* Since  $f_{\theta_m}^i \rightarrow f_\theta^i$  for every  $i$  pointwise by Assumption 2,  $Y_m^n \rightsquigarrow Y^n$  (see Proof of Theorem 2.1). Thus, by Slutsky's theorem,  $(\theta_m, Y_m^n) \rightsquigarrow (\theta, Y^n)$ . The result now follows from the continuous mapping theorem and Theorem 2.1.  $\square$

**Lemma D.2.** *If Assumption 2 holds, then  $\mathbb{E}_\theta\{s_n(\theta; Y^n)\} = 0$  for all  $\theta \in \Theta$ .*

*Proof.* Let  $\gamma^n$  denote the product measure  $\otimes_{i=1}^n \gamma_i$ . Pick a sequence  $t_m \downarrow 0$  as  $m \rightarrow \infty$  and use the mean value theorem, applicable by Assumption 2, to write for some  $\tilde{t}_m \in [0, t_m]$ ,

$$\begin{aligned} 0 &= t_m^{-1} \int \{f_{\theta+t_m e_j}(y^n) - f_\theta(y^n)\} \gamma^n(dy^n) \\ &= \int \nabla_j f_{\theta+\tilde{t}_m e_j}(y^n) \gamma^n(dy^n) \\ &= \int s_{nj}(\theta + \tilde{t}_m e_j; y^n) f_{\theta+\tilde{t}_m e_j}(y^n) \gamma^n(dy^n) \\ &= \mathbb{E}\{s_{nj}(\theta_m, Y_m^n)\}, \end{aligned}$$

where  $\theta_m = \theta + \tilde{t}_m e_j \rightarrow \theta$  as  $m \rightarrow \infty$  and  $Y_m^n$  has the distribution indexed by  $\theta_m$ . By Slutsky's theorem,  $(\theta_m, Y_m^n) \rightsquigarrow (\theta, Y^n)$ , where  $Y^n$  has the distribution indexed by  $\theta$ . Thus, by Assumption 2 and the continuous mapping theorem,  $s_{nj}(\theta_m, Y_m^n) \rightsquigarrow s_{nj}(\theta, Y^n)$ . Moreover, by Assumption 2 there exists an  $M < \infty$  such that  $\mathbb{E}\{s_{nj}(\theta_m; Y_m^n)^2\} \leq M$  for all large enough  $m$ . Thus, the sequence  $\{s_{nj}(\theta_m, Y_m^n)\}$  is uniformly integrable and, consequently,  $0 = \mathbb{E}\{s_{nj}(\theta_m; Y_m^n)\} \rightarrow \mathbb{E}\{s_{nj}(\theta; Y^n)\}$ , which completes the proof.  $\square$

## E Proofs of results in main text

*Proof of Lemma 2.2.* The assumptions of the lemma imply  $T_n(\cdot; \cdot)$  is continuous on  $\{\theta : \mathcal{I}(\theta) > 0\} \times \mathcal{Y}^n$ . They also say we may, for any critical  $\theta$  and  $y^n \in \mathcal{Y}^n$ , unambiguously define  $T_n(\theta; y^n) = \lim_{m \rightarrow \infty} T_n(\theta_m; y^n)$ , where  $\{\theta_m\}$  is any sequence of non-critical points tending to  $\theta$ ; Assumption 5 says at least one such sequence exists. To verify this extension is continuous on  $\Theta \times \mathcal{Y}^n$ , let instead  $\{\theta_m\} \in \Theta$  be an arbitrary sequence, possibly including critical points, tending to  $\theta$ . Let also  $\{y_m^n\} \in \mathcal{Y}^n$  be an arbitrary sequence tending to  $y^n$ . By the assumptions of the lemma, we can find, for every fixed  $m$ , a non-critical  $\tilde{\theta}_m$  such that

$$|T_n(\theta_m; y_m^n) - T_n(\tilde{\theta}_m; y_m^n)| \leq 1/m \quad \text{and} \quad \|\theta_m - \tilde{\theta}_m\| \leq 1/m.$$

Thus, by the triangle inequality,

$$|T_n(\theta_m; y_m^n) - T_n(\theta; y^n)| \leq 1/m + |T_n(\tilde{\theta}_m; y_m^n) - T_n(\theta; y^n)|,$$

which tends to zero by the assumptions of the lemma since  $\{\tilde{\theta}_m\}$  is a sequence of non-critical points tending to  $\theta$ .  $\square$

*Proof of Lemma 2.5.* We first prove Equation (5) implies Equation (4) in the main text. For contradiction, suppose (5) holds and that there exist a compact  $C \subseteq \Theta$  and an  $\epsilon > 0$  such that, for infinitely many  $n$ ,  $\sup_{\theta \in C} |\mathbb{P}_\theta \{\theta \in \mathcal{R}_n(\alpha)\} - (1 - \alpha)| > \epsilon$ . Let  $N$  be the set of such  $n$  and pick, for every  $n \in N$ , a  $\theta_n \in C$  such that  $|\mathbb{P}_{\theta_n} \{\theta_n \in \mathcal{R}_n(\alpha)\} - (1 - \alpha)| > \epsilon$ . Because  $C$  is compact, it is bounded and hence  $\{\theta_n : n \in N\}$  is a bounded sequence. Thus, it contains a convergent subsequence. But by (5), along this subsequence,  $T_n(\theta_n; Y_n^n) \rightsquigarrow \chi_d^2$ ; in particular, since  $\chi_d^2$  has a continuous cumulative distribution function,  $\mathbb{P}_{\theta_n} \{\theta_n \in \mathcal{R}_n(\alpha)\} = \mathbb{P}\{T_n(\theta_n; Y_n^n) \leq q_{d,1-\alpha}\} \rightarrow 1 - \alpha$  along the subsequence, which is the desired contradiction.

To prove Equation (4) implies Equation (5) in the main text, note that if  $\theta_n \rightarrow \theta$ , then for all large enough  $n$ ,  $\theta_n$  is in a compact neighborhood  $C$  of  $\theta$ . Thus, for those  $n$  and any  $\alpha \in (0, 1)$ ,  $|\mathbb{P}\{T_n(\theta_n; Y_n^n) \leq q_{d,1-\alpha}\} - (1 - \alpha)| = |\mathbb{P}_{\theta_n} \{\theta_n \in \mathcal{R}_n(\alpha)\} - (1 - \alpha)| \leq \sup_{\theta \in C} |\mathbb{P}_\theta \{\theta \in \mathcal{R}_n(\alpha) - (1 - \alpha)\}|$ , which tends to zero by (4). Thus, since the range of  $\alpha \mapsto q_{d,1-\alpha}$  is  $(0, \infty)$ , the cumulative distribution function of  $T_n(\theta_n; Y_n^n)$  tends to that of  $\chi_d^2$  at every point in  $\mathbb{R}$ , which completes the proof.  $\square$

*Proof of Lemma 3.7.* Differentiating  $\log f_\theta(y_i)$  with respect to  $\psi$  gives  $s_\psi^i(\theta; y_i, X_i) = X_i^\top \Sigma_i^{-1}(y_i - X_i \psi)$ . Differentiating this with respect to  $\lambda$  and taking expectations shows  $\mathcal{I}^i(\theta)$  is block-diagonal. The trailing  $d_2 \times d_2$  block is  $\mathcal{I}_\psi^i(\theta) = \text{cov}_\theta \{s_\psi^i(\theta; Y_i, X_i)\} = \mathbb{E}(X_i^\top \Sigma_i^{-1} X_i)$ , which is positive definite for all  $\theta$  since  $\underline{e}(\Sigma) \geq \sigma^2 > 0$  and  $\underline{e}\{\mathbb{E}(X_i^\top X_i)\} > 0$  by assumption; the result follows.  $\square$

*Proof of Lemma 3.8.* For  $j = 1, \dots, d_1$ , let

$$\zeta_j^i(\theta; y_i, X_i) = \text{tr} \left\{ \Sigma_i^{-1} H_j^i - \Sigma_i^{-1} (y_i - X_i \psi) (y_i - X_i \psi)^\top \Sigma_i^{-1} H_j^i \right\},$$

which are the first  $d_1$  elements of  $\xi^i(\theta; y_i, X_i)$  defined in the proof of Theorem 3.9. In particular, for  $\lambda_j > 0$ ,  $\zeta_j^i(\theta; y_i, X_i) = s_j^i(\theta; y_i, X_i) / \lambda_j$ , and hence the claim to be proved is equivalent to, for any  $v \in \mathbb{R}^{d_1}$ ,

$$\bar{e}(\Sigma_i)^{-2} \underline{e}(Z_i^\top Z_i)^2 \max_j (v_j)^2 \leq \frac{1}{2} \text{var}_\theta \{v^\top \zeta^i(\theta; Y_i, X_i) \mid X_i\} \leq r_i \underline{e}(\Sigma_i)^{-2} \bar{e}(Z_i^\top Z_i)^2 \max_j (v_j)^2.$$

With  $G_i = \sum_{j=1}^{d_1} v_j H_j^i \in \mathbb{R}^{r_i \times r_i}$ , we have

$$v^\top \zeta^i(\theta; Y_i, X_i) = \text{tr} \left[ \left\{ \Sigma_i^{-1} - \Sigma_i^{-1} (Y_i - X_i \psi) (Y_i - X_i \psi)^\top \Sigma_i^{-1} \right\} G_i \right].$$

Thus, applying the well-known expression for the variance of a quadratic form in multivariate

normal vectors (Seber and Lee, 2003, Theorem 1.6),

$$\begin{aligned}\text{var}_\theta \{v^\top \zeta^i(\theta; Y_i, X_i) \mid X_i\} &= \text{var}_\theta [\text{tr} \{ \Sigma_i^{-1} (Y_i - X_i \psi) (Y_i - X_i \psi)^\top \Sigma_i^{-1} G_i \} \mid X_i] \\ &= \text{var}_\theta [(Y_i - X_i \psi)^\top \Sigma_i^{-1} G_i \Sigma_i^{-1} (Y_i - X_i \psi) \mid X_i] \\ &= 2 \text{tr}[(\Sigma_i^{-1/2} G_i \Sigma_i^{-1/2})^2].\end{aligned}$$

We start with the lower bound. Observe that since  $\Sigma_i^{-1/2} G_i \Sigma_i^{-1/2}$  is symmetric, its eigenvalues are real, and hence the eigenvalues of its square are non-negative as the squares of real numbers. Thus, the trace upper bounds the maximum eigenvalue, and hence  $\text{var}_\theta \{v^\top \zeta^i(\theta; Y_i, X_i) \mid X_i\}$  is lower bounded by

$$2 \|(\Sigma_i^{-1/2} G_i \Sigma_i^{-1/2})^2\| \geq 2 \underline{e}(\Sigma_i^{-1}) \|\Sigma_i^{-1/2} G_i^2 \Sigma_i^{-1/2}\| \geq 2 \underline{e}(\Sigma_i^{-1})^2 \bar{e}(G_i^2).$$

Now write

$$G_i = \sum_{j=1}^{d_1} \sum_{k \in [j]} v_j Z_i^k (Z_i^k)^\top = \sum_{k=1}^q v_{j(k)} Z_i^k (Z_i^k)^\top = Z_i \tilde{V} Z_i^\top,$$

where  $v_{j(k)}$  is the  $v_j$  scaling  $Z_i^k (Z_i^k)^\top$  in the double sum and  $\tilde{V}$  is diagonal with the elements of  $v$  on the diagonal, ordered so that the last equality holds. Then  $\|G_i^2\| = \|Z_i \tilde{V} Z_i^\top Z_i \tilde{V} Z_i^\top\| \geq \underline{e}(Z_i^\top Z_i) \|Z_i \tilde{V}^2 Z_i^\top\|$ . The last norm is  $\|Z_i \tilde{V}^2 Z_i^\top\| = \bar{e}(Z_i \tilde{V}^2 Z_i^\top) = \max_{\|b\|=1} b^\top Z_i \tilde{V}^2 Z_i^\top b$  which by considering  $b = Z_i^l / \|Z_i^l\|$  is lower bounded by, for every  $l = 1, \dots, q$ ,

$$\left( \frac{Z_i^l}{\|Z_i^l\|} \right)^\top \sum_{k=1}^q v_{j(k)}^2 Z_i^k (Z_i^k)^\top \left( \frac{Z_i^l}{\|Z_i^l\|} \right) \geq v_{j(l)} \|Z_i^l\|^2 \geq v_{j(l)}^2 \min_k \|Z_i^k\|^2.$$

Thus, because it holds for every  $l$  it holds for  $l \in \arg \max_k v_{j(k)}^2$ , and the proof of the lower bound is completed by observing  $\|Z_i^k\|^2 = e_k^\top Z_i^\top Z_i e_k \geq \underline{e}(Z_i^\top Z_i)$ . For the upper bound, note

$$2 \text{tr}[(\Sigma_i^{-1/2} G_i \Sigma_i^{-1/2})^2] \leq 2 r_i \|\Sigma_i^{-1}\|^2 \|G_i\|^2 \leq 2 r_i \|\Sigma_i^{-1}\|^2 \|Z_i\|^4 \|\tilde{V}\|^2,$$

which is equal to the stated upper bound and hence the proof is completed.  $\square$

*Proof of Theorem 3.10.* The claim about  $\mathcal{R}_n^\lambda(\alpha)$  is almost immediate from Theorem 3.9 and the fact that  $\mathcal{I}_n(\theta)$  is block diagonal so we omit the proof. To prove the second claim, observe

that  $T_n^\lambda(\lambda; \psi, Y^n, X^n)$  is equal to

$$\left\{ n^{-1/2} \sum_{i=1}^n \zeta^i(\theta; Y_i, X_i)^\top \right\} \text{cov}_\theta \{ \zeta^1(\theta; Y_1, X_1) \}^{-1} \left\{ n^{-1/2} \sum_{i=1}^n \zeta^i(\theta; Y_i, X_i) \right\},$$

where  $\zeta^i$  is defined in the proof of Lemma 3.8. Let  $C(\theta)$  be the covariance matrix in the middle term. We showed in the proof of Lemma 3.8 that  $C(\theta)$  is positive definite at any  $\theta$ ; in particular,  $v^\top C(\theta)v \geq 2 \max_j v_j^2 \bar{e}(\Sigma_1)^{-2} \underline{e}(Z_1^\top Z_1)^2$ . Moreover, it is straightforward to show  $C$  is continuous using uniform integrability of  $\{ \zeta^1(\theta_m; Y_{m1}, X_{m1}) \zeta^1(\theta_m; Y_{m1}, X_{m1})^\top \}$ , where  $(Y_{m1}, X_{m1})$  has the distribution indexed by a  $\theta_m$  tending to some  $\theta$ ; the arguments are very similar to those in the proof of Theorem 2.1 and hence omitted. Thus, it suffices (Billingsley, 1999, Theorems 2.7 and 3.1) to show

$$\left\| n^{-1/2} \sum_{i=1}^n \zeta^i(\lambda_n; \psi_n, Y_{ni}, X_{ni}) - n^{-1/2} \sum_{i=1}^n \zeta^i(\lambda_n; \hat{\psi}_n, Y_{ni}, X_{ni}) \right\| = o_{\mathbf{P}}(1),$$

where  $(Y_{ni}, X_{ni})$  has the distribution indexed by  $\theta_n$ . We show the equivalent result that every element of the vector in the norm is  $o_{\mathbf{P}}(1)$ . The  $j$ th element is

$$n^{-1/2} \sum_{i=1}^n \left\{ (Y_{ni} - X_{ni}\psi_n)^\top \Omega_{nj} (Y_{ni} - X_{ni}\psi_n) - (Y_{ni} - X_{ni}\hat{\psi}_n)^\top \Omega_{nj} (Y_{ni} - X_{ni}\hat{\psi}_n) \right\},$$

where  $\Omega_{nj} = \Sigma_n^{-1} H_j \Sigma_n^{-1}$ . Let  $\varepsilon_{ni} = Y_{ni} - X_{ni}\psi_n \sim \mathcal{N}(0, \Sigma_n)$  to get that the last display is equal to

$$n^{-1/2} \sum_{i=1}^n \left[ \varepsilon_{ni}^\top \Omega_{nj} \varepsilon_{ni} - \{ \varepsilon_{ni} + X_{ni}(\psi_n - \hat{\psi}_n) \}^\top \Omega_{nj} \{ \varepsilon_{ni} + X_{ni}(\psi_n - \hat{\psi}_n) \} \right],$$

which in turn is equal to

$$-n^{-1/2} 2(\psi_n - \hat{\psi}_n)^\top \sum_{i=1}^n X_{ni}^\top \Omega_{nj} \varepsilon_{ni} - n^{-1/2} (\psi_n - \hat{\psi}_n)^\top \left( \sum_{i=1}^n X_{ni}^\top \Omega_{nj} X_{ni} \right) (\psi_n - \hat{\psi}_n).$$

Thus, since  $\|\psi_n - \hat{\psi}_n\| = O_{\mathbf{P}}(1/\sqrt{n})$  it suffices to show that

$$\left\| n^{-1} \sum_{i=1}^n X_{ni}^\top \Omega_{nj} \varepsilon_{ni} \right\| = o_{\mathbf{P}}(1) \quad \text{and} \quad \left\| n^{-1} \sum_{i=1}^n X_{ni}^\top \Omega_{nj} X_{ni} \right\| = O_{\mathbf{P}}(1).$$

For the former we show the elements are  $o_P(1)$  and for the latter it suffices, since the matrix in the norm is positive semi-definite, to show the diagonal elements are  $O_P(1)$ . First, then, condition on  $\{X_1, \dots, X_n\}$ , apply Chebyshev's inequality, and take expectations to get, for any  $s \geq 0$  and standard basis vector  $e_l$ ,

$$\begin{aligned} \mathbb{P} \left\{ \left| e_l^\top n^{-1} \sum_{i=1}^n X_{ni}^\top \Omega_{nj} \varepsilon_{ni} \right| \geq s \right\} &\leq \frac{1}{s^2 n^2} \mathbb{E} \left( \sum_{i=1}^n e_l^\top X_{ni}^\top \Omega_{nj} \Sigma_n \Omega_{nj} X_{ni} e_l \right) \\ &\leq \frac{1}{s^2 n} \|H_j\|^2 \sigma^{-6} \mathbb{E}(\|X_1\|^2), \end{aligned}$$

which tends to zero since  $\|H_j\| \leq \|Z^\top Z\|$  and  $\mathbb{E}(\|X_1\|^2)$  are bounded by assumption. The second holds since, for any standard basis vector  $e_l$ ,  $e_l^\top X_{ni}^\top \Omega_{nj} X_{ni} e_l \leq \|\Omega_{nj}\| e_l^\top X_{ni}^\top X_{ni} e_l$ ,  $\|\Omega_{nj}\| \leq \|H_j\| \|\Sigma^{-1}\| \leq \|H_j\| \sigma^{-4}$ , and  $n^{-1} \sum_{i=1}^n e_l^\top X_{ni}^\top X_{ni} e_l \rightarrow e_l^\top \mathbb{E}(X_1^\top X_1) e_l < \infty$  by the law of large numbers.  $\square$

## F Additional simulations

Figure C summarizes the results of a Monte Carlo experiment with 10,000 replications and compares coverage probabilities for our method with  $\psi$  known and  $\psi$  estimated, i.e. a nuisance parameter. Other than that, the settings are like those for producing Figure 2 in the main text. Notably, coverage is slightly higher when estimating  $\psi$ . Nevertheless, coverage is near-nominal in all settings and the differences between known and estimated  $\psi$  are especially small for larger  $n$ .

Figure D here is also similar to Figure 2 in the main text, but here  $\sigma$  is treated as unknown. In the simulations, the unknown  $\sigma = 1$  and coverage probabilities are for a range of  $(\lambda_1, \lambda_2, \sigma) = (\lambda_1, \lambda_2, 1)$  where the values of  $\lambda_1 = \lambda_2$  are on the horizontal axis in Figure D. All confidence regions use the chi-square distribution with 3 degrees of freedom as reference.

## References

- Billingsley, P. (1999). *Convergence of Probability Measures*. Wiley series in probability and statistics. Probability and statistics section. Wiley, New York, second edition.
- Ferguson, T. S. (1996). *A Course in Large Sample Theory*. Springer US, Boston, MA.

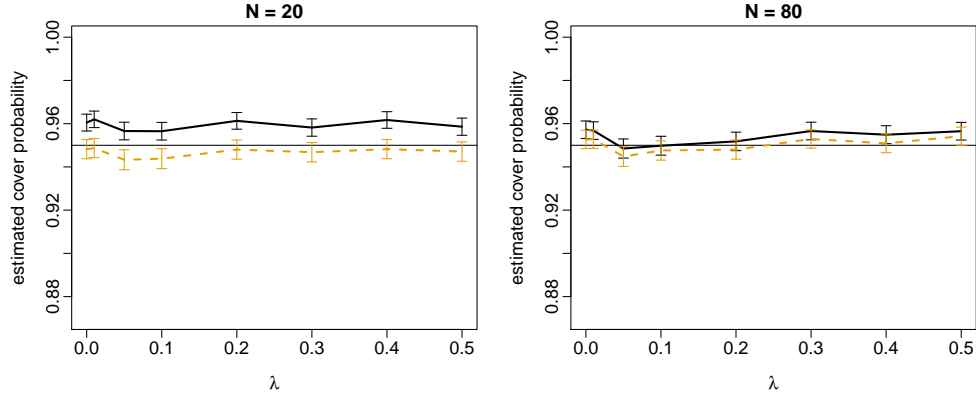

Figure C: Monte Carlo estimates of coverage probabilities of confidence regions from inverting the modified score with  $\psi$  estimated (solid) or known (dashed). The straight horizontal line indicates the nominal 0.95 coverage probability and vertical bars denote  $\pm 2$  times Monte Carlo standard errors.

Knudson, C., Benson, S., Geyer, C., and Jones, G. (2021). Likelihood-based inference for generalized linear mixed models: Inference with the R package glmm. *Stat*, 10(1):e339.

Riviere, M.-K., Ueckert, S., and Mentré, F. (2016). An MCMC method for the evaluation of the Fisher information matrix for non-linear mixed effect models. *Biostatistics*, 17(4):737–750.

Seber, G. A. F. and Lee, A. J. (2003). *Linear Regression Analysis*. Wiley series in probability and statistics. Wiley-Interscience, Hoboken, N.J, 2nd ed edition.

Smyth, G. K. (1998). Numerical integration. *Encyclopedia of biostatistics*, pages 3088–3095.

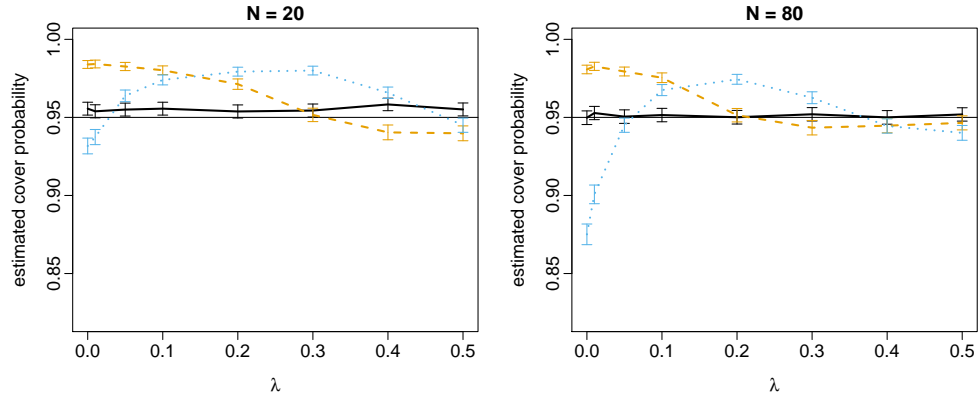

Figure D: Monte Carlo estimates of coverage probabilities of confidence regions from inverting the modified score (solid), likelihood ratio (dashed), and Wald (dotted) test-statistics. The straight horizontal line indicates the nominal 0.95 coverage probability and vertical bars denote  $\pm 2$  times Monte Carlo standard errors.
